# Supplementary material for: Quantum Fluctuations in Noether's Theorem
Source: arXiv:2611.08906 source file (2026-11-06)
Supplement: Supplementary file 1 [file Supplementary_Information.tex]

\documentclass[onecolumn,superscriptaddress,pra]{revtex4}
\usepackage{amsmath}
\usepackage{amssymb}
\usepackage{graphicx}
\usepackage{bm}

\begin{document}

\title{Supplementary Information: Quantum Fluctuations in Noether's Theorem.}

\author{J. A. Crosse}
\email{jac32@nyu.edu}
\affiliation{New York University Shanghai, 1555 Century Avenue, Pudong, Shanghai, 200122, China.}
\affiliation{NYU-ECNU Institute of Physics at NYU Shanghai, 3663 Zhongshan Road North, Shanghai, 200062, China.}

\maketitle

\section{Lagrangian Mechanics}

\subsection{The Euler-Lagrange Equation}

The motion of a particle is given by the path that extremizes the action, $\delta S = 0$. The action is given by
\begin{equation}
S = \int_{t_i}^{t_f}dt\, L(x,\dot{x}),
\end{equation}
where the Lagrangian, $L=K(\dot{x})-U(x)$, is the difference between the kinetic, $K$, and potential, $U$, energies. Varying the action leads to
\begin{align}
\delta S &= \int_{t_i}^{t_f}dt\, \delta L(x,\dot{x}),\nonumber\\
&= \int_{t_i}^{t_f}dt\,\left[\frac{\partial  L}{\partial x}\delta x + \frac{\partial  L}{\partial \dot{x}}\delta \dot{x}\right],\nonumber\\
&= \int_{t_i}^{t_f}dt\,\left[\frac{\partial  L}{\partial x}\delta x + \frac{d}{dt}\left(\frac{\partial  L}{\partial \dot{x}}\delta x\right) - \frac{d}{dt}\left(\frac{\partial  L}{\partial \dot{x}}\right)\delta x\right],\nonumber\\
&= \int_{t_i}^{t_f}dt\,\left[\frac{\partial  L}{\partial x}\delta x - \frac{d}{dt}\left(\frac{\partial  L}{\partial \dot{x}}\right)\delta x\right] + \left.\frac{\partial  L}{\partial \dot{x}}\delta x\right|_{t_i}^{t_f}.
\end{align}
As the variation at the initial and final points is zero, $\delta x(t_i) = \delta x(t_f) = 0$, the final boundary term vanishes and one has
\begin{equation}
\int_{t_i}^{t_f}dt\,\left[\frac{\partial  L}{\partial x} - \frac{d}{dt}\left(\frac{\partial  L}{\partial \dot{x}}\right)\right]\delta x  = 0,
\end{equation}
which, if this is to be true for all $t_i$ and $t_f$, implies
\begin{equation}
\frac{\partial  L}{\partial x} - \frac{d}{dt}\left(\frac{\partial  L}{\partial \dot{x}}\right) = 0.
\end{equation}
This is the Euler-Lagrange equation, which defines the classical path of the system.

\subsection{Noether's Theorem}

Noether's Theorem states that, if the action is invariant up to a boundary term, then there is a conserved quantity.
\begin{equation}
\delta S = \int_{t_i}^{t_f}dt\,\left[\frac{\partial  L}{\partial x}\delta x + \frac{\partial  L}{\partial \dot{x}}\delta \dot{x}\right] = \Lambda(t)\bigg|_{t_i}^{t_f}.
\label{dx}
\end{equation}
With some rearrangement one finds
\begin{gather}
\int_{t_i}^{t_f}dt\,\left[\frac{\partial  L}{\partial x}\delta x + \frac{\partial  L}{\partial \dot{x}}\delta \dot{x}\right] - \Lambda(t)\bigg|_{t_i}^{t_f} = 0,\nonumber\\
\int_{t_i}^{t_f}dt\,\left[\frac{\partial  L}{\partial x}\delta x + \frac{\partial  L}{\partial \dot{x}}\delta \dot{x} - \frac{d\Lambda}{dt} \right] = 0,\nonumber\\
\int_{t_i}^{t_f}dt\,\left[\frac{\partial  L}{\partial x}\delta x + \frac{d}{dt}\left(\frac{\partial  L}{\partial \dot{x}}\delta x\right) - \frac{d}{dt}\left(\frac{\partial  L}{\partial \dot{x}}\right)\delta x - \frac{\partial \Lambda}{\partial t} \right] = 0,\nonumber\\
\int_{t_i}^{t_f}dt\,\left\{\frac{d}{dt}\left[\left(\frac{\partial  L}{\partial \dot{x}}\delta x\right)  - \Lambda\right] + \left[\frac{\partial  L}{\partial x} - \frac{d}{dt}\left(\frac{\partial  L}{\partial \dot{x}}\right)\right]\delta x\right\} = 0.
\label{1}
\end{gather}
The second term vanishes via the Euler-Lagrange equation. If, again, the integral is to be vanishes for all $t_i$ and $t_f$, this implies that the first term must also vanish. Therefore
\begin{equation}
\frac{d}{dt}\left[\left(\frac{\partial  L}{\partial \dot{x}}\delta x\right)  - \Lambda\right]=0,
\end{equation}
which implies that the quantity in square brackets does not change with time and, hence, the quantity
\begin{equation}
J_{cl} = \left(\frac{\partial  L}{\partial \dot{x}}\delta x\right)  - \Lambda,
\end{equation}
is conserved. $J_{cl}$, is called the Noether's current.

\subsection{Conservation of Energy}

If the action is not an explicit function of time then a time translation, $t' = t + \epsilon$, leaves the action invariant. In this situation we have
\begin{equation}
\delta x = \frac{1}{\epsilon}\left[x(t') - x(t)\right] = \frac{1}{\epsilon}\left[x(t + \epsilon) - x(t)\right] =\frac{1}{\epsilon}\left[x(t) + \epsilon\displaystyle\frac{dx}{dt} - x(t)\right] = \dot{x}.
\end{equation}
From the second line of Eq. \eqref{1}, above, we see that
\begin{equation}
\frac{d\Lambda}{dt}  = \frac{\partial  L}{\partial x}\delta x + \frac{\partial  L}{\partial \dot{x}}\delta \dot{x},
\end{equation}
and hence
\begin{align}
\frac{d\Lambda}{dt}   &= \frac{\partial  L}{\partial x}\delta x + \frac{\partial  L}{\partial \dot{x}}\delta \dot{x},\nonumber\\
&= \frac{\partial  L}{\partial x} \dot{x} + \frac{\partial  L}{\partial \dot{x}} \ddot{x},\nonumber\\
&= \frac{\partial  L}{\partial x}\frac{\partial x}{\partial t} + \frac{\partial  L}{\partial \dot{x}}\frac{\partial \dot{x}}{\partial t} = \frac{dL}{dt}.
\end{align}
The conserved current is therefore found to be
\begin{equation}
J_{cl} = \left(\frac{\partial  L}{\partial \dot{x}}\delta x\right)  - \Lambda = \left(\frac{\partial  L}{\partial \dot{x}}\dot{x}\right)  - L = H,
\end{equation}
i.e. the Hamiltonian or the total energy.

\section{Quantum Fluctuations in Lagrangian Mechanics}

\subsection{Conserved Current Fluctuations}

The derivation of Noether's theorem assumed the particle travelled along the classical path, as defined by the solutions to the Euler-Lagrange equation. If the particle doesn't then the second term in the last line of Eq. \eqref{1} does not vanish and one has
\begin{equation}
\int_{t_i}^{t_f}dt\,\left\{\frac{d}{dt}\left[\left(\frac{\partial  L}{\partial \dot{x}}\delta x\right)  - \Lambda\right] + \left[\frac{\partial  L}{\partial x} - \frac{d}{dt}\left(\frac{\partial  L}{\partial \dot{x}}\right)\right]\delta x\right\} = 0.
\end{equation}
If one writes 
\begin{equation}
\frac{dF}{dt} = \left[\frac{\partial  L}{\partial x} - \frac{d}{dt}\left(\frac{\partial  L}{\partial \dot{x}}\right)\right]\delta x,
\label{F}
\end{equation}
one obtains
\begin{equation}
\int_{t_i}^{t_f}dt\,\left\{\frac{d}{dt}\left[\left(\frac{\partial  L}{\partial \dot{x}}\delta x\right)  - \Lambda\right] = \frac{dF}{dt}\right\} = 0,
\end{equation}
and now, if the integral is to vanish for all $t_i$ and $t_f$, one has
\begin{equation}
\frac{d}{dt}\left[\left(\frac{\partial  L}{\partial \dot{x}}\delta x\right)  - \Lambda + F\right]= 0
\end{equation}
and, hence, the conserved current becomes
\begin{equation}
J = \left(\frac{\partial  L}{\partial \dot{x}}\delta x\right) + F - \Lambda = J_{cl} + F.
\end{equation}
Along the classical path $F=0$. Off the classical path this is not necessarily the case. Thus, $F$ represents a quantum fluctuation of the energy due to the particle not following the classical path.

\subsection{Energy Fluctuations}

To find an expression for the quantum fluctuations, $F$, one can expand the Lagrangian about the classical path (parameterized by $x_{cl}$ and $\dot{x}_{cl}$)
\begin{multline}
L[x_{cl} + y,\dot{x}_{cl} + \dot{y}] = L[x_{cl},\dot{x}_{cl}] + \left(y\left.\frac{\partial L[x,\dot{x}]}{\partial x}\right|_{x=x_{cl}}+\dot{y}\left.\frac{\partial L[x,\dot{x}]}{\partial \dot{x}}\right|_{x=x_{cl}}\right)\\
+ \frac{1}{2}\left(y^2\left.\frac{\partial^2 L[x,\dot{x}]}{\partial x^2}\right|_{x=x_{cl}}+2y\dot{y}\left.\frac{\partial^2 L[x,\dot{x}]}{\partial \dot{x}\partial x}\right|_{x=x_{cl}}+\dot{y}^2\left.\frac{\partial^2 L[x,\dot{x}]}{\partial \dot{x}^2}\right|_{x=x_{cl}}\right) + \cdots
\end{multline}
The zeroth order term is just the Lagrangian along the classical path and, hence, obeys the Euler-Lagrange equation and so its contribution to the quantum fluctuations vanishes. The first order term is the variation of the Lagrangian (action). The classical path extremizes the action so this term is, by definition, zero along the classical path. The second order term is the lowest order term that contributes to the quantum fluctuations.

If the Lagrangian is bilinear or quadratic in $x$ and $\dot{x}$ then the second order derivatives will result in two times the constant prefactor for that term, which cancels the factor of half from the Taylor expansion. Hence, the effect of the expansion is to replace the variables $x$ and $\dot{x}$ in the Lagrangian with $y$ and $\dot{y}$, 
\begin{equation}
L^{(2)} = L[y,\dot{y}].
\label{L2}
\end{equation}
Furthermore, this term will be the highest order term in the expansion. All higher order terms will vanish. 

One can compute the quantum fluctuations by substituting \eqref{L2} into \eqref{F} and changing variables $x\rightarrow x_{cl} + y$ where $x_{cl}$ acts as a constant.
\begin{align}
\frac{dF}{dt} &= \left[\frac{\partial  L^{(2)}}{\partial y} - \frac{d}{dt}\left(\frac{\partial  L^{(2)}}{\partial \dot{y}}\right)\right]\delta y,\nonumber\\
&=\left[\frac{\partial L[y,\dot{y}]}{\partial y} - \frac{d}{dt}\left(\frac{\partial L[y,\dot{y}]}{\partial \dot{y}}\right)\right]\dot{y},
\end{align}
where in the second line we have used $\delta y = \dot{y}$, which is the substitution required for a time symmetric Lagrangian and, hence, energy fluctuations. One can simplify this expression by noting that the total derivative of the Lagrangian is
\begin{equation}
\frac{dL}{dt} = \frac{\partial L}{\partial y}\frac{dy}{dt}+\frac{\partial L}{\partial \dot{y}}\frac{d\dot{y}}{dt}.
\end{equation}
Thus, one can write
\begin{align}
\frac{dF}{dt} &= \left[\frac{\partial L}{\partial y} - \frac{d}{dt}\left(\frac{\partial L}{\partial \dot{y}}\right)\right]\frac{dy}{dt},\nonumber\\
&= \left[\frac{\partial L}{\partial y}\frac{dy}{dt} - \frac{d}{dt}\left(\frac{\partial L}{\partial \dot{y}}\right)\frac{dy}{dt}\right],\nonumber\\
&= \left[\frac{dL}{dt} - \frac{\partial L}{\partial \dot{y}}\frac{d\dot{y}}{dt} - \frac{d}{dt}\left(\frac{\partial L}{\partial \dot{y}}\right)\frac{dy}{dt}\right],\nonumber\\
&= \frac{d}{dt}\left[L - \frac{\partial L}{\partial \dot{y}}\dot{y}\right],\nonumber\\
&= \frac{d}{dt}\left[-H(y)\right],
\end{align}
where $H(y)$ is the Hamiltonian for the system but in terms of the variable $y$, the deviation from the classical path. Thus, we can see that the energy fluctuations are given by
\begin{equation}
F = -H(y),
\end{equation}
which is minus the functional expression for the Hamiltonian evaluated at the distance from the classical path.

\section{Example: Energy Fluctuations of the Harmonic Oscillator}

As a concrete example we can compute the energy fluctuations of the Harmonic oscillator. The Lagrangian for the Harmonic oscillator is given by
\begin{equation}
L = \frac{1}{2}m\dot{x}(t)^2 - \frac{1}{2}m\omega^2 x(t)^2,
\end{equation}
and, hence, it is quadratic in both $x(t)$ and $\dot{x}(t)$. To find the non-classical fluctuation, $F$, one can perform a functional expansion of the Lagrangian about the classical path
\begin{equation}
L[x_{cl} + y] = L[x_{cl}] + \int dt'\,y(t')\left.\frac{\delta L[x]}{\delta x(t')}\right|_{x=x_{cl}} + \frac{1}{2}\int dt''\int dt'\,y(t'')y(t')\left.\frac{\delta^{2} L[x]}{\delta x(t'')\delta x(t')}\right|_{x=x_{cl}} + \cdots
\end{equation}
The first order term we would expect to vanish since this defines the classical path
\begin{align}
\frac{\delta L[x]}{\delta x(t')} &= \frac{\delta}{\delta x(t')}\left[\frac{1}{2}m\dot{x}(t)^2 - \frac{1}{2}m\omega^2x(t)^2\right],\nonumber\\
&= \left[m\dot{x}(t)\frac{d}{dt}\frac{\delta x(t)}{\delta x(t')} - m\omega^2x(t)\frac{\delta x(t)}{\delta x(t')}\right],\nonumber\\
&= \left[m\dot{x}(t)\frac{d}{dt}\delta(t-t') - m\omega^2x(t)\delta(t-t')\right],
\end{align}
and, hence,
\begin{align}
\int dt'\,y(t')\left.\frac{\delta L[x]}{\delta x(t')}\right|_{x=x_{cl}} &= \int dt'\,y(t')\left[m\dot{x}(t)\frac{d}{dt}\delta(t-t') - m\omega^2x(t)\delta(t-t')\right]_{x=x_{cl}},\nonumber\\
 &= \int dt'\,y(t')\left[-m\ddot{x}(t)\delta(t-t') - m\omega^2x(t)\delta(t-t')\right]_{x=x_{cl}},\nonumber\\
&= -m\,y(t)\left[\ddot{x}_{cl}(t) + \omega^2x_{cl}(t)\right].
\end{align}
The term in square brackets is just the Euler-Lagrange equation of motion for the harmonic oscillator. As this is evaluated along the classical path this term vanishes identically as expected. 
\newpage

The second order term is computed as follows
\begin{align}
\frac{\delta^{2} L[x]}{\delta x(t'')\delta x(t')} &= \frac{\delta^{2}}{\delta x(t'')\delta x(t')}\left[\frac{1}{2}m\dot{x}(t)^2 - \frac{1}{2}m\omega^2x(t)^2\right],\nonumber\\
&= \frac{\delta^{2}}{\delta x(t'')}\left[m\dot{x}(t)\frac{d}{dt}\delta(t-t') - m\omega^2x(t)\delta(t-t')\right],\nonumber\\
&= \left[m\frac{d}{dt}\delta(t-t'')\frac{d}{dt}\delta(t-t') - m\omega^2\delta(t-t'')\delta(t-t')\right].
\end{align}
Thus
\begin{align}
&\frac{1}{2}\int dt''\int dt'\,y(t'')y(t')\left.\frac{\delta^{2} L[x]}{\delta x(t'')\delta x(t')}\right|_{x=x_{cl}}\nonumber\\
&\qquad = \frac{1}{2}\int dt''\int dt'\,y(t'')y(t')\left[m\frac{d}{dt}\delta(t-t'')\frac{d}{dt}\delta(t-t') - m\omega^2\delta(t-t'')\delta(t-t')\right],\nonumber\\
&\qquad = \frac{m}{2}\left[\dot{y}(t)^2 - \omega^2y(t)^2\right],
\end{align}
which is the usual second order expansion of the path that is found in evaluation of the Feynman path integral for the harmonic oscillator. Again, substituting this back into Eq. \eqref{F} and noting that the variable has change from $x$ to $x_{cl}+y$ where $x_{cl}$ is a constant path we find
\begin{align}
\frac{dF}{dt} &= \left[\frac{\partial  L^{(2)}}{\partial y} - \frac{d}{dt}\left(\frac{\partial  L^{(2)}}{\partial \dot{y}}\right)\right]\delta x ,\nonumber\\
&= \left[-m\ddot{y}(t) - m\omega^2y(t)\right]\dot{y},\nonumber\\
&= \frac{d}{dt}\left[-\frac{1}{2}m\dot{y}(t)^2 - \frac{1}{2}m\omega^2y(t)^2\right],\nonumber\\
&= \frac{d}{dt}\left[-H(y)\right].
\end{align}
Thus
\begin{equation}
F = -H(y),
\end{equation}
and we find that the energy fluctuations are given by minus the functional expression for the Hamiltonian evaluated at the distance from the classical path as expected.

\section{Expectation Value of the Energy Fluctuations of the Harmonic Oscillator}

To find the average energy fluctuations (which is equivalent to the variance of the actual energy) over a time, $\Delta t$, on can use the path integral formulism to evaluate the matrix element of the energy fluctuations between time $t=0$ and time $t=\Delta t$ and then take the time average over that interval
\begin{equation}
\Delta E = \frac{1}{\Delta t}\int_{0}^{\Delta t}dt\,\langle F(t) \rangle = \frac{1}{\Delta t}\int_{0}^{\Delta t}dt\,\left\{\frac{\displaystyle\int\mathcal{D}y\, F\, e^{iS/\hbar}}{\displaystyle\int\mathcal{D}y\,e^{iS/\hbar}}\right\}.
\end{equation}
As the denominator is the usual harmonic oscillator transition amplitude, which is independent of $t$ (it is only a function of $\Delta t$), one can write
\begin{equation}
\Delta E = \frac{\displaystyle\int\mathcal{D}y\,\left\{\frac{1}{\Delta t}\int_{0}^{\Delta t}dt\, F(t)\right\} e^{iS/\hbar}}{\displaystyle\int\mathcal{D}y\,e^{iS/\hbar}}.
\label{dE}
\end{equation}
Substituting in the expression for $F(t)$ and the expansion of the action, $S$, about the classical path into Eq. \eqref{dE} gives
\begin{equation}
\Delta E = \frac{e^{iS_{cl}/\hbar}\displaystyle\int\mathcal{D}y\,\left\{-\frac{m}{2\Delta t}\int_{0}^{\Delta t}dt\,\left[\dot{y}(t)^2 + \omega^2y(t)^2\right]\right\} e^{\displaystyle i\frac{m}{2\hbar}\int_{0}^{\Delta t}dt\,\left[\dot{y}(t)^2 - \omega^2y(t)^2\right]}}{\displaystyle\int\mathcal{D}y\,e^{iS/\hbar}}.
\end{equation}
where $S_{cl}$ is the action along the classical path. We can evaluate the path integral in the usual way by substituting in the Fourier series expansion for $y$
\begin{gather}
y = \sum_{n=1}^{N}a_n\sin\left(\frac{n\pi t}{\Delta t}\right),\\
\dot{y} = \sum_{n=1}^{N}a_n\left(\frac{n\pi}{\Delta t}\right)\cos\left(\frac{n\pi t}{\Delta t}\right).
\end{gather}
which we write as a finite series of $N$ terms but will eventually take $N\rightarrow\infty$. Thus, one has
\begin{equation}
\int_{0}^{\Delta t}dt\,\left[\dot{y}(t)^2 \pm \omega^2y(t)^2\right] =\int_{0}^{\Delta t}dt\,\sum_{n=1}^{N}\sum_{j=1}^{N}a_na_j\left[\left(\frac{n\pi}{\Delta t}\right)\left(\frac{j\pi}{\Delta t}\right)\cos\left(\frac{n\pi t}{\Delta t}\right)\cos\left(\frac{j\pi t}{\Delta t}\right) \pm \omega^2\sin\left(\frac{n\pi t}{\Delta t}\right)\sin\left(\frac{j\pi t}{\Delta t}\right)\right].\\
\label{int}
\end{equation}
As the Fourier terms are orthogonal
\begin{gather}
\int_{0}^{\Delta t}\cos\left(\frac{n\pi t}{\Delta t}\right)\cos\left(\frac{j\pi t}{\Delta t}\right) = \frac{\Delta t}{2}\delta_{nj},\\
\int_{0}^{\Delta t}\sin\left(\frac{n\pi t}{\Delta t}\right)\sin\left(\frac{j\pi t}{\Delta t}\right) = \frac{\Delta t}{2}\delta_{nj},
\end{gather}
the expression in Eq. \eqref{int} collapses to
\begin{align}
\int_{0}^{\Delta t}dt\,\left[\dot{y}(t)^2 \pm \omega^2y(t)^2\right] &= \int_{0}^{\Delta t}dt\,\sum_{n=1}^{N}\sum_{j=1}^{N}a_na_j\left[\left(\frac{n\pi}{\Delta t}\right)\left(\frac{j\pi}{\Delta t}\right)\cos\left(\frac{n\pi t}{\Delta t}\right)\cos\left(\frac{j\pi t}{\Delta t}\right) \pm \omega^2\sin\left(\frac{n\pi t}{\Delta t}\right)\sin\left(\frac{j\pi t}{\Delta t}\right)\right],\nonumber\\
&=\sum_{n=1}^{N}\sum_{j=1}^{N}a_na_j\left[\left(\frac{n\pi}{\Delta t}\right)\left(\frac{j\pi}{\Delta t}\right)\frac{\Delta t}{2}\delta_{nj} \pm \omega^2\frac{\Delta t}{2}\delta_{nj}\right],\nonumber\\
&=\frac{\Delta t}{2}\sum_{j}a_j^2\left[\left(\frac{j\pi}{\Delta t}\right)^2 \pm \omega^2\right].
\end{align}
Substituting these expressions back into the path integral and changing variables to the Fourier coefficients and remembering that for $N+1$ time slices there are $N-1$ independent variables (the points at $t=0$ and $t=\Delta t$ are fixed) and hence $a_{j}=0$ for $j > N-1$ leads to 
\begin{align}
\Delta E &= \lim_{N\rightarrow \infty}\frac{e^{iS_{cl}/\hbar}\displaystyle J_N \left(\frac{1}{2\pi i\hbar \varepsilon}\right)^{N/2}\int da_1 \cdots da_{N-1} \,\left\{-\frac{m}{4}\sum_{j=1}^{N-1}a_j^2\left[\left(\frac{j\pi}{\Delta t}\right)^2 + \omega^2\right]\right\} e^{\displaystyle i\frac{m\Delta t}{4\hbar}\sum_{n=1}^{N-1}a_n^2\left[\left(\frac{n\pi}{\Delta t}\right)^2 - \omega^2\right]}}{\displaystyle\int\mathcal{D}y\,e^{iS/\hbar}},\nonumber\\
&= \lim_{N\rightarrow \infty}\frac{e^{iS_{cl}/\hbar}\displaystyle J_N \left(\frac{1}{2\pi i\hbar \varepsilon}\right)^{N/2}\int da_1 \cdots da_{N-1} \left\{-\frac{m}{4}\sum_{j=1}^{N-1}a_j^2\left[\left(\frac{j\pi}{\Delta t}\right)^2 + \omega^2\right]\right\}\prod_{n=1}^{N-1} e^{\displaystyle i\frac{m\Delta t}{4\hbar}\left[\left(\frac{n\pi}{\Delta t}\right)^2 - \omega^2\right]a_n^2}}{\displaystyle\int\mathcal{D}y\,e^{iS/\hbar}},
\end{align}
where $J_N$ is the Jacobian of the variable change and $\varepsilon = \Delta t/N$ is the finite interval between steps in the discrete path. Each term in the sum over $j$ consists of a product of $N-2$ Gaussian $I_0$ integrals (when $j\neq n$) and one Gaussian $I_2$ integral (when $j=n$)
\begin{gather}
I_{0} = \int_{-\infty}^{\infty}dx\,e^{-\alpha x^2} = \sqrt{\frac{\pi}{\alpha}},\\
I_{2} = \int_{-\infty}^{\infty}dx\,x^2\,e^{-\alpha x^2} = \frac{1}{2\alpha}\sqrt{\frac{\pi}{\alpha}}.
\end{gather}
Evaluating the Gaussian integrals leads to
\begin{align}
\Delta E &= \lim_{N\rightarrow \infty}\frac{e^{iS_{cl}/\hbar}\displaystyle J_N \left(\frac{1}{2\pi i\hbar \varepsilon}\right)^{N/2}\left\{-\frac{m}{4}\sum_{j=1}^{N-1}\left[\left(\frac{j\pi}{\Delta t}\right)^2 + \omega^2\right]\right\}\frac{1}{2i\frac{m\Delta t}{4\hbar}\left[\left(\frac{j\pi}{\Delta t}\right)^2 - \omega^2\right]}\prod_{n=1}^{N-1}\left(\frac{\pi}{i\frac{m\Delta t}{4\hbar}\left[\left(\frac{n\pi}{\Delta t}\right)^2 - \omega^2\right]}\right)^{1/2}}{\displaystyle\int\mathcal{D}y\,e^{iS/\hbar}}\nonumber\\
&= \lim_{N\rightarrow \infty}\frac{i\hbar}{2\Delta t}\sum_{j=1}^{N-1}\frac{\displaystyle\left[\left(\frac{j\pi}{\Delta t}\right)^2 + \omega^2\right]}{\displaystyle\left[\left(\frac{j\pi}{\Delta t}\right)^2 - \omega^2\right]}\frac{\left\{e^{iS_{cl}/\hbar}\displaystyle J_N \left(\frac{1}{2\pi i\hbar \varepsilon}\right)^{N/2}\prod_{n=1}^{N-1}\left(\frac{\pi}{i\frac{m\Delta t}{4\hbar}\left[\left(\frac{n\pi}{\Delta t}\right)^2 - \omega^2\right]}\right)^{1/2}\right\}}{\displaystyle\int\mathcal{D}y\,e^{iS/\hbar}}.
\end{align}
The expression in the brackets in the numerator is exactly the expression for the transition amplitude of the Harmonic oscillator
\begin{equation}
\int\mathcal{D}y\,e^{iS/\hbar} = e^{iS_{cl}/\hbar}\displaystyle J_N \left(\frac{1}{2\pi i\hbar \varepsilon}\right)^{N/2}\prod_{n=1}^{N-1}\left(\frac{\pi}{i\frac{m\Delta t}{4\hbar}\left[\left(\frac{n\pi}{\Delta t}\right)^2 - \omega^2\right]}\right)^{1/2},
\end{equation}
and hence cancels with the path integral in the denominator. Thus we have
\begin{equation}
\Delta E = \lim_{N\rightarrow \infty}\frac{i\hbar}{2\Delta t}\sum_{j=1}^{N-1}\frac{\displaystyle\left[\left(\frac{j\pi}{\Delta t}\right)^2 + \omega^2\right]}{\displaystyle\left[\left(\frac{j\pi}{\Delta t}\right)^2 - \omega^2\right]}.
\end{equation}
The sum can be split into two parts by adding and subtracting a factor of $\omega^2$ to the numerator
\begin{equation}
\Delta E = \lim_{N\rightarrow \infty}\frac{i\hbar}{2\Delta t}\sum_{j=1}^{N-1}\frac{\displaystyle\left[\left(\frac{j\pi}{\Delta t}\right)^2 - \omega^2 + 2\omega^2\right]}{\displaystyle\left[\left(\frac{j\pi}{\Delta t}\right)^2 - \omega^2\right]} = \lim_{N\rightarrow \infty}\frac{i\hbar}{2\Delta t}\left\{\sum_{j=1}^{N-1}1 + \sum_{j=1}^{N-1}\frac{\displaystyle 2\omega^2}{\displaystyle\left[\left(\frac{j\pi}{\Delta t}\right)^2 - \omega^2\right]}\right\}.
\label{sum}
\end{equation}
At this point some care is needed. The evaluation of the summations and the limit do not commute. If one evaluates the limit first then one obtains an extra factor of $i\hbar/2\Delta t$ in the solution. In studies of the Casimir force between two perfectly conducting plates terms of this form sometimes appear depending on the method used to analyze the effect. They are often referred to as contact terms and quantify the self energy of each individual plate. These terms are often disregarded as they are not a function of the plate separation and hence do not contribute to the Casimir Force itself. In this case we can avoid the appearance of this term completely by evaluating the summations first. The first sum easily evaluates to
\begin{equation}
\sum_{j=1}^{N-1}1 = N-1.
\end{equation}
The factor of $N$ clearly diverges when the limit as $N\rightarrow\infty$ is taken. This corresponds to an infinite vacuum energy. The second sum evaluates to a rather complicated expression involving the digamma function, $\psi^{(0)}(z)$,
\begin{equation}
\sum_{j=1}^{N-1}\frac{\displaystyle 2\omega^2}{\displaystyle\left[\left(\frac{j\pi}{\Delta t}\right)^2 - \omega^2\right]} = 1-\omega\Delta t\cot\left(\omega\Delta t\right)+ \frac{\omega\Delta t}{\pi}\left[\psi^{(0)}\left(N - \frac{\omega\Delta t}{\pi}\right) - \psi^{(0)}\left(N + \frac{\omega\Delta t}{\pi}\right)\right].
\end{equation}
However, in the limit as $N\rightarrow\infty$ the digamma functions cancel. Thus, finite part of the average vacuum energy fluctuations becomes
\begin{equation}
\Delta E = -\frac{i\hbar\omega}{2}\cot\left(\omega\Delta t\right). 
\label{E}
\end{equation}
Note that the factor of `$1$' from the second summation is canceled by the factor of `$-1$' from the first summation. This removes the contact term.

If one expands the expression in Eq. \eqref{E} for small $\Delta t$ one obtains
\begin{equation}
\Delta E \approx -\frac{i\hbar}{2\Delta t} + \frac{i\hbar}{6}\omega^2\Delta t + \mathcal{O}\left(\Delta t^3\right),
\end{equation}
which to leading order recovers the energy-time uncertainty relation up to an irrelevant complex phase
\begin{equation}
\Delta E \Delta t \approx -i\frac{\hbar}{2}.
\end{equation}
We can find the average vacuum energy fluctuations in the long time limit by adding a small imaginary element then taking the time interval to infinity, $\Delta t \rightarrow \infty(1-i\epsilon)$
\begin{equation}
\Delta E = \lim_{\Delta t \rightarrow \infty(1-i\epsilon)}-\frac{i\hbar\omega}{2}\cot\left(\omega\Delta t\right) = \frac{\hbar\omega}{2},
\end{equation}
which is the zero-point energy for a single Harmonic oscillator.


\end{document}
